# Supplementary material for: User Identification via Free Roaming Eye Tracking Data
Source: arXiv:2403.09415 source file (2024-03-14)
Supplement: Supplementary file 1 [file Appendix.tex]

%\section{Appendix}
%%
%%
%\begin{table}[!h]
%\caption{AGE GROUP 0 – 40M 40F}
%\label{1}
%\begin{tabular}{ccccc}
%\toprule
%Results & ROI feature   & Classifier & Pipeline feature & Classifier \\ \midrule
%2min    & 60.7 ± 2.0 \% & logreg     & 60.1 ± 1.9 \%    & svm        \\
%1min    & 63.6 ± 2.3 \% & logreg     & 61.7 ± 1.8 \%    & rf         \\
%40sec   & 61.1 ± 2.2 \% & logreg     & 61.4 ± 1.9 \%    & rf         \\
%20sec   & 56.1 ± 2.3 \% & logreg     & 60.1 ± 2.0 \%    & rf         \\
%12sec   & 57.6 ± 1.8 \% & logreg     & 60.0 ± 1.7 \%    & rf         \\
%\bottomrule
%\end{tabular}
%\end{table}
%
%\begin{table}[!h]
%\caption{AGE GROUP 1 – 40M 40F}
%\label{1}
%\begin{tabular}{lllll}
%\toprule
%Results & ROI feature   & Classifier & Pipeline feature & Classifier \\ \midrule
%2min    & 57.8 ± 1.6 \% & logreg     & 64.2 ± 1.4 \%    & rf         \\
%1min    & 55.4 ± 1.7 \% & nb         & 61.8 ± 1.6 \%    & rf         \\
%40sec   & 57.1 ± 1.8 \% & logreg     & 62.0 ± 1.6 \%    & rf         \\
%20sec   & 54.8 ± 1.9 \% & rf         & 63.6 ± 1.6 \%    & rf         \\
%12sec   & 55.9 ± 1.6 \% & logreg     & 61.3 ± 1.7 \%    & rf       \\ 
%\bottomrule
%\end{tabular}
%\end{table}
%
%\begin{table}[!h]
%\caption{AGE GROUP 2 – 40M 40F}
%\label{1}
%\begin{tabular}{ccccc}
%\toprule
%Results & ROI feature  & Classifier & Pipeline feature & Classifier \\ \midrule
%2min    & 61.5 ± 1.8 \% & svm        & 54.1 ± 1.6 \%     & rf         \\
%1min    & 59.0 ± 1.8 \% & svm        & 54.5 ± 1.5 \%     & rf         \\
%40sec   & 62.4 ± 1.6 \% & logreg     & 54.1 ± 1.4 \%     & svm        \\
%20sec   & 58.1 ± 1.5 \% & logreg     & 53.9 ± 1.3 \%     & svm        \\
%12sec   & 64.5 ± 1.6 \% & logreg     & 54.4 ± 1.3 \%     & logreg    \\
%\bottomrule
%\end{tabular}
%\end{table}
%
%
%
%
%
%
%
%
%
%
%
%
%
%
%
%
%
%
%
%
%
%
%
%
%
%
%
%
%
%
%
%
%
%
%
%
%
%
%
%
%
%%\subsection{GOF Results}
%%% Please add the following required packages to your document preamble:
%%% \usepackage{multirow}
%%% \usepackage{graphicx}
%%%
%%\begin{table*}[]
%%\centering
%%\begin{tabular*}{0.78\textwidth}{@{\extracolsep{\fill}}|c|c|c|c|c|c|c|}
%%
%%\hline
%%\multicolumn{7}{|c|}{Age Group 0 results}                                                                                                                                                                         \\ \hline
%%Time duration                                                                  & Feature Type & LogReg                 & SVM                    & RF                     & Naive Bayes   & RBFN                   \\ \hline
%%\multirow{2}{*}{\begin{tabular}[c]{@{}c@{}}12 second\\ duration\end{tabular}}  & ROI          & 57.6 ± 0.8 \%          & 58.5 ± 0.7 \%          & 57.3 ± 0.8 \%          & 56.2 ± 0.8 \% & \textbf{59.1 ± 0.7 \%} \\ \cline{2-7} 
%%                                                                               & Pipeline     & 60.9 ± 0.8 \%          & 59.0 ± 0.6 \%          & \textbf{61.6 ± 0.6 \%} & 52.6 ± 0.3 \% & 58.4 ± 0.6 \%          \\ \hline
%%\multirow{2}{*}{\begin{tabular}[c]{@{}c@{}}20 second \\ duration\end{tabular}} & ROI          & \textbf{56.3 ± 0.7 \%} & 55.3 ± 0.7 \%          & 55.4 ± 0.8 \%          & 54.8 ± 0.7 \% & 56.2 ± 0.7 \%          \\ \cline{2-7} 
%%                                                                               & Pipeline     & 58.1 ± 0.7 \%          & 56.7 ± 0.6 \%          & \textbf{59.5 ± 0.7 \%} & 53.4 ± 0.4 \% & 56.7 ± 0.6 \%          \\ \hline
%%\multirow{2}{*}{\begin{tabular}[c]{@{}c@{}}40 second\\ duration\end{tabular}}  & ROI          & \textbf{59.3 ± 0.7 \%} & 57.5 ± 0.6 \%          & 58.7 ± 0.7 \%          & 57.8 ± 0.9 \% & 57.0 ± 0.7 \%          \\ \cline{2-7} 
%%                                                                               & Pipeline     & 60.9 ± 0.7 \%          & 61.0 ± 0.6 \%          & \textbf{61.8 ± 0.8 \%} & 53.8 ± 0.4    & 61.6 ± 0.7 \%          \\ \hline
%%\multirow{2}{*}{\begin{tabular}[c]{@{}c@{}}1 minute\\ duration\end{tabular}}   & ROI          & \textbf{58.8 ± 0.6 \%} & 57.7 ± 0.7 \%          & 56.5 ± 0.7 \%          & 57.9 ± 0.6 \% & 57.7 ± 0.7 \%          \\ \cline{2-7} 
%%                                                                               & Pipeline     & 62.5 ± 0.7             & 61.8 ± 0.6 \%          & \textbf{62.7 ± 0.8}    & 51.8 ± 0.2    & 61.5 ± 0.6             \\ \hline
%%\multirow{2}{*}{\begin{tabular}[c]{@{}c@{}}2 minute\\ duration\end{tabular}}   & ROI          & 58.2 ± 0.6 \%          & \textbf{60.9 ± 0.7 \%} & 57.7 ± 0.8 \%          & 57.0 ± 0.6 \% & 59.5 ± 0.7 \%          \\ \cline{2-7} 
%%                                                                               & Pipeline     & \textbf{63.7 ± 0.6 \%} & 60.9 ± 0.6 \%          & 63.4 ± 0.7 \%          & 52.5 ± 0.3 \% & 62.1 ± 0.6 \%          \\ \hline
%%\end{tabular*}
%%\caption{Results for Age group 0}
%%\label{AgeGroup0}
%%\end{table*}
%%
%%%%%%%%%%%%%%%%%%%%%%%%%
%%%% Please add the following required packages to your document preamble:
%%%% \usepackage{multirow}
%%%% \usepackage{graphicx}
%%\begin{table*}[]
%%\centering
%%\begin{tabular*}{0.78\textwidth}{@{\extracolsep{\fill}}|c|c|c|c|c|c|c|}
%%\hline
%%\multicolumn{7}{|c|}{Age Group 1 results}                                                                                                                                                                \\ \hline
%%Time duration                                                                  & Feature Type & LogReg                 & SVM                    & RF                     & Naive Bayes   & RBFN          \\ \hline
%%\multirow{2}{*}{\begin{tabular}[c]{@{}c@{}}12 second\\ duration\end{tabular}}  & ROI          & \textbf{56.7 ± 1.0 \%} & 55.2 ± 1.0 \%          & 55.3 ± 0.9 \%          & 55.3 ± 0.9 \% & 56.0 ± 1.1 \% \\ \cline{2-7} 
%%                                                                               & Pipeline     & 62.6 ± 0.9 \%          & 60.5 ± 0.8 \%          & \textbf{63.8 ± 1.0 \%} & 54.2 ± 0.7 \% & 60.6 ± 0.9 \% \\ \hline
%%\multirow{2}{*}{\begin{tabular}[c]{@{}c@{}}20 second \\ duration\end{tabular}} & ROI          & \textbf{56.0 ± 1.1 \%} & 51.5 ± 0.9 \%          & 53.6 ± 1.0 \%          & 53.6 ± 1.0 \% & 49.8 ± 0.2 \% \\ \cline{2-7} 
%%                                                                               & Pipeline     & \textbf{62.0 ± 1.0 \%} & 55.0 ± 0.7 \%          & 60.2 ± 1.0 \%          & 53.6 ± 0.9 \% & 55.0 ± 0.7 \% \\ \hline
%%\multirow{2}{*}{\begin{tabular}[c]{@{}c@{}}40 second\\ duration\end{tabular}}  & ROI          & \textbf{59.2 ± 1.1 \%} & 52.5 ± 1.0 \%          & 54.3 ± 1.0 \%          & 56.2 ± 0.8 \% & 57.0 ± 1.1 \% \\ \cline{2-7} 
%%                                                                               & Pipeline     & \textbf{63.4 ± 0.9 \%} & 60.9 ± 0.9 \%          & 62.7 ± 1.0 \%          & 54.4 ± 1.0 \% & 62.3 ± 0.8 \% \\ \hline
%%\multirow{2}{*}{\begin{tabular}[c]{@{}c@{}}1 minute\\ duration\end{tabular}}   & ROI          & \textbf{58.1 ± 1.0 \%} & 54.8 ± 1.1 \%          & 55.3 ± 1.0 \%          & 55.3 ± 1.0 \% & 57.0 ± 1.0 \% \\ \cline{2-7} 
%%                                                                               & Pipeline     & 63.4 ± 0.9             & 62.1 ± 0.8 \%          & \textbf{64.1 ± 1.0}    & 52.3 ± 0.5    & 62.0 ± 0.8    \\ \hline
%%\multirow{2}{*}{\begin{tabular}[c]{@{}c@{}}2 minute\\ duration\end{tabular}}   & ROI          & 60.0 ± 1.0 \%          & \textbf{58.8 ± 1.0 \%} & 55.2 ± 1.0 \%          & 58.3 ± 1.1 \% & 61.0 ± 0.9 \% \\ \cline{2-7} 
%%                                                                               & Pipeline     & \textbf{66.2 ± 0.9 \%} & 62.2 ± 0.8 \%          & 65.2 ± 1.0 \%          & 52.9 ± 0.5 \% & 62.1 ± 0.8 \% \\ \hline
%%\end{tabular*}%
%%
%%\caption{Results for Age Group 1}
%%\label{AgeGroup1}
%%\end{table*}
%%
%%
%%%%%%%%%%%%%%%%%%%%%%%%%%%%%%%%%%%%%%%
%%
%%% Please add the following required packages to your document preamble:
%%% \usepackage{multirow}
%%% \usepackage{graphicx}
%%\begin{table*}[]
%%\centering
%%\begin{tabular*}{0.78\textwidth}{@{\extracolsep{\fill}}|c|c|c|c|c|c|c|}
%%\hline
%%\multicolumn{7}{|c|}{Age Group 2 results}                                                                                                                                                                \\ \hline
%%Time duration                                                                  & Feature Type & LogReg                 & SVM                    & RF                     & Naive Bayes   & RBFN          \\ \hline
%%\multirow{2}{*}{\begin{tabular}[c]{@{}c@{}}12 second\\ duration\end{tabular}}  & ROI          & \textbf{64.5 ± 1.6 \%} & 62.1 ± 1.5 \%          & 61.8 ± 1.6 \%          & 61.6 ± 1.5 \% & 63.9 ± 1.4 \% \\ \cline{2-7} 
%%                                                                               & Pipeline     & \textbf{54.4 ± 1.3 \%} & 50.5 ± 1.1 \%          & 53.2 ± 1.5 \%          & 49.9 ± 1.1 \% & 48.5 ± 1.4 \% \\ \hline
%%\multirow{2}{*}{\begin{tabular}[c]{@{}c@{}}20 second \\ duration\end{tabular}} & ROI          & \textbf{58.1 ± 1.5 \%} & 57.4 ± 1.4 \%          & 51.5 ± 1.7 \%          & 57.8 ± 1.2 \% & 55.6 ± 1.5 \% \\ \cline{2-7} 
%%                                                                               & Pipeline     & 52.6 ± 1.4 \%          & 53.9 ± 1.3 \%          & 51.1 ± 1.4 \%          & 52.2 ± 0.9 \% & 49.9 ± 1.8 \% \\ \hline
%%\multirow{2}{*}{\begin{tabular}[c]{@{}c@{}}40 second\\ duration\end{tabular}}  & ROI          & \textbf{62.4 ± 1.6 \%} & 58.2 ± 1.5 \%          & 59.5 ± 1.6 \%          & 56.4 ± 1.3 \% & 56.1 ± 1.8 \% \\ \cline{2-7} 
%%                                                                               & Pipeline     & 52.2 ± 1.4 \%          & \textbf{54.1 ± 1.4 \%} & 53.2 ± 1.6 \%          & 52.8 ± 0.6 \% & 53.1 ± 1.2 \% \\ \hline
%%\multirow{2}{*}{\begin{tabular}[c]{@{}c@{}}1 minute\\ duration\end{tabular}}   & ROI          & 57.8 ± 1.5 \%          & \textbf{59.0 ± 1.8 \%} & 57.8 ± 1.5 \%          & 55.5 ± 1.6 \% & 57.4 ± 1.7 \% \\ \cline{2-7} 
%%                                                                               & Pipeline     & 53.1 ± 1.3 \%          & 51.6 ± 0.9 \%          & \textbf{54.5 ± 1.5 \%} & 54.5 ± 1.5 \% & 52.4 ± 1.2 \% \\ \hline
%%\multirow{2}{*}{\begin{tabular}[c]{@{}c@{}}2 minute\\ duration\end{tabular}}   & ROI          & 58.8 ± 1.6 \%          & \textbf{61.5 ± 1.8 \%} & 52.2 ± 1.2 \%          & 57.4 ± 1.5 \% & 51.5 ± 1.5 \% \\ \cline{2-7} 
%%                                                                               & Pipeline     & 51.4 ± 1.1 \%          & 51.2 ± 1.1 \%          & \textbf{54.1 ± 1.6 \%} & 50.4 ± 0.7 \% & 52.8 ± 1.1 \% \\ \hline
%%\end{tabular*}%
%%
%%\caption{Results for Age Group 2}
%%\label{AgeGroup2}
%%\end{table*}
%%
%%%%%%%%%%%%%%%%%%%%%%%%%%%%%%%%%%%%%%%%
%%%\newpage
%%%\cleardoublepage
%%% Please add the following required packages to your document preamble:
%%% \usepackage{multirow}
%%% \usepackage{graphicx}
%%\begin{table*}[]
%%\centering
%%\begin{tabular*}{0.78\textwidth}{@{\extracolsep{\fill}}|c|c|c|c|c|c|c|}
%%\hline
%%\multicolumn{7}{|c|}{Age Group 3 results}                                                                                                                                                                \\ \hline
%%Time duration                                                                  & Feature Type & LogReg                 & SVM                    & RF                     & Naive Bayes   & RBFN          \\ \hline
%%\multirow{2}{*}{\begin{tabular}[c]{@{}c@{}}12 second\\ duration\end{tabular}}  & ROI          & 35.5 ± 3.2 \%          & \textbf{56.5 ± 2.8 \%} & 42.5 ± 2.6 \%          & 33.5 ± 3.1 \% & 36.0 ± 3.5 \% \\ \cline{2-7} 
%%                                                                               & Pipeline     & 52.5 ± 2.2 \%          & 53.5 ± 1.4 \%          & \textbf{56.0 ± 3.0 \%} & 50.0 ± 0.7 \% & 50.5 ± 1.3 \% \\ \hline
%%\multirow{2}{*}{\begin{tabular}[c]{@{}c@{}}20 second \\ duration\end{tabular}} & ROI          & 49.5 ± 4.1 \%          & \textbf{58.0 ± 2.2 \%} & 54.0 ± 2.9 \%          & 47.0 ± 3.9 \% & 48.5 ± 3.5 \% \\ \cline{2-7} 
%%                                                                               & Pipeline     & 51.0 ± 1.6 \%          & 49.0 ± 1.2 \%          & \textbf{63.5 ± 3.1 \%} & 47.0 ± 1.3 \% & 51.0 ± 1.2 \% \\ \hline
%%\multirow{2}{*}{\begin{tabular}[c]{@{}c@{}}40 second\\ duration\end{tabular}}  & ROI          & \textbf{58.0 ± 3.5 \%} & 49.5 ± 0.5 \%          & 55.5 ± 3.5 \%          & 45.5 ± 3.5 \% & 40.5 ± 2.7 \% \\ \cline{2-7} 
%%                                                                               & Pipeline     & 54.0 ± 2.0 \%          & 53.0 ± 1.7 \%          & \textbf{56.5 ± 2.7 \%} & 50.0 ± 0.0 \% & 53.0 ± 2.1 \% \\ \hline
%%\multirow{2}{*}{\begin{tabular}[c]{@{}c@{}}1 minute\\ duration\end{tabular}}   & ROI          & \textbf{54.5 ± 3.5 \%} & 50.0 ± 0.0 \%          & 48.5 ± 2.9 \%          & 52.0 ± 3.1 \% & 48.0 ± 3.6 \% \\ \cline{2-7} 
%%                                                                               & Pipeline     & 51.0 ± 1.0 \%          & 52.5 ± 1.6 \%          & \textbf{56.5 ± 3.4 \%} & 50.0 ± 0.0 \% & 54.5 ± 2.0 \% \\ \hline
%%\multirow{2}{*}{\begin{tabular}[c]{@{}c@{}}2 minute\\ duration\end{tabular}}   & ROI          & 58.0 ± 3.6 \%          & \textbf{50.0 ± 0.0 \%} & 53.0 ± 2.5 \%          & 54.5 ± 3.2 \% & 52.0 ± 2.6 \% \\ \cline{2-7} 
%%                                                                               & Pipeline     & 50.5 ± 1.1 \%          & 55.0 ± 1.9 \%          & \textbf{57.0 ± 2.5 \%} & 50.0 ± 0.0 \% & 52.0 ± 2.1 \% \\ \hline
%%\end{tabular*}%
%%
%%\caption{Results for Age Group 3}
%%\label{AgeGroup3}
%%\end{table*}
%%
%%%%%%%%%%%%%%%%%%%%%%%%%%%
%%% Please add the following required packages to your document preamble:
%%% \usepackage{multirow}
%%% \usepackage{graphicx}
%%\begin{table*}[]
%%\centering
%%\begin{tabular*}{0.78\textwidth}{@{\extracolsep{\fill}}|c|c|c|c|c|c|c|}
%%\hline
%%\multicolumn{7}{|c|}{New - Age Group 1 results}                                                                                                                                                          \\ \hline
%%Time duration                                                                  & Feature Type & LogReg              & SVM           & RF                     & Naive Bayes         & RBFN                \\ \hline
%%\multirow{2}{*}{\begin{tabular}[c]{@{}c@{}}12 second\\ duration\end{tabular}}  & ROI          & \textbf{55.9 ± 0.9} & 52.0 ± 0.9    & 51.9 ± 1.0             & 54.9 ± 1.0          & 55.7 ± 0.9          \\ \cline{2-7} 
%%                                                                               & Pipeline     & 57.8 ± 1.1          & 53.4 ± 0.7 \% & \textbf{60.6 ± 0.9 \%} & 51.9 ± 0.6          & 56.4 ± 0.8          \\ \hline
%%\multirow{2}{*}{\begin{tabular}[c]{@{}c@{}}20 second \\ duration\end{tabular}} & ROI          & 55.3 ± 1.0          & 53.3 ± 0.8 \% & 53.7 ± 1.0             & \textbf{56.1 ± 0.7} & 54.5 ± 0.9          \\ \cline{2-7} 
%%                                                                               & Pipeline     & 57.3 ± 0.9          & 51.9 ± 0.7 \% & \textbf{58.8 ± 0.7 \%} & 50.3 ± 0.2          & 56.3 ± 1.0          \\ \hline
%%\multirow{2}{*}{\begin{tabular}[c]{@{}c@{}}40 second\\ duration\end{tabular}}  & ROI          & 55.9 ± 0.9          & 53.6 ± 0.9 \% & 54.9 ± 0.9 \%          & \textbf{56.2 ± 1.0} & 52.5 ± 1.0          \\ \cline{2-7} 
%%                                                                               & Pipeline     & 57.1 ± 1.1          & 53.0 ± 0.6    & \textbf{60.1 ± 0.9 \%} & 50.0 ± 0.0          & 58.6 ± 1.0          \\ \hline
%%\multirow{2}{*}{\begin{tabular}[c]{@{}c@{}}1 minute\\ duration\end{tabular}}   & ROI          & 55.4 ± 1.0          & 54.2 ± 1.0 \% & 56.5 ± 1.2             & 55.4 ± 1.0          & \textbf{56.8 ± 0.9} \\ \cline{2-7} 
%%                                                                               & Pipeline     & 59.1 ± 1.0          & 57.5 ± 0.9    & \textbf{62.0 ± 0.9 \%} & 53.5 ± 0.6          & 59.2 ± 0.9          \\ \hline
%%\multirow{2}{*}{\begin{tabular}[c]{@{}c@{}}2 minute\\ duration\end{tabular}}   & ROI          & 55.2 ± 1.1          & 53.9 ± 0.8 \% & 53.8 ± 1.1             & 51.6 ± 0.9          & \textbf{56.6 ± 0.9} \\ \cline{2-7} 
%%                                                                               & Pipeline     & 59.5 ± 1.0          & 59.1 ± 0.9    & \textbf{63.0 ± 1.0}    & 52.8 ± 0.6          & 59.7 ± 0.9          \\ \hline
%%\end{tabular*}%
%%
%%\caption{Results for New Age Group 1}
%%\label{NewAgeGroup1}
%%\end{table*}
%%
%%%%%%%%%%%%%%%%%%%%%%%%%
%%
%%% Please add the following required packages to your document preamble:
%%% \usepackage{multirow}
%%% \usepackage{graphicx}
%%\begin{table*}[]
%%\centering
%%\begin{tabular*}{0.78\textwidth}{@{\extracolsep{\fill}}|c|c|c|c|c|c|c|}
%%\hline
%%\multicolumn{7}{|c|}{New - Age Group 2 results}                                                                                                                                                           \\ \hline
%%Time duration                                                                  & Feature Type & LogReg              & SVM                    & RF                     & Naive Bayes & RBFN                \\ \hline
%%\multirow{2}{*}{\begin{tabular}[c]{@{}c@{}}12 second\\ duration\end{tabular}}  & ROI          & \textbf{62.8 ± 1.9} & 60.5 ± 2.0 \%          & 49.2 ± 1.9 \%          & 58.2 ± 1.6  & 56.7 ± 1.6          \\ \cline{2-7} 
%%                                                                               & Pipeline     & 48.3 ± 1.2          & 52.0 ± 1.3             & \textbf{54.0 ± 2.1 \%} & 50.0 ± 0.0  & 45.2 ± 1.5          \\ \hline
%%\multirow{2}{*}{\begin{tabular}[c]{@{}c@{}}20 second \\ duration\end{tabular}} & ROI          & 57.0 ± 1.9          & \textbf{58.3 ± 1.7 \%} & 51.3 ± 1.7 \%          & 54.3 ± 1.8  & 56.0 ± 1.6          \\ \cline{2-7} 
%%                                                                               & Pipeline     & 50.2 ± 1.0          & 51.7 ± 0.9             & \textbf{58.0 ± 1.8 \%} & 50.0 ± 0.0  & 52.2 ± 1.4          \\ \hline
%%\multirow{2}{*}{\begin{tabular}[c]{@{}c@{}}40 second\\ duration\end{tabular}}  & ROI          & 57.8 ± 2.2          & 58.0 ± 1.5 \%          & 53.3 ± 1.7 \%          & 52.2 ± 1.9  & \textbf{60.0 ± 1.5} \\ \cline{2-7} 
%%                                                                               & Pipeline     & 44.3 ± 1.0          & 52.7 ± 1.5 \%          & \textbf{56.0 ± 2.1}    & 50.0 ± 0.0  & 52.2 ± 1.9          \\ \hline
%%\multirow{2}{*}{\begin{tabular}[c]{@{}c@{}}1 minute\\ duration\end{tabular}}   & ROI          & 56.0 ± 1.9          & \textbf{59.5 ± 2.1 \%} & 59.3 ± 1.6 \%          & 53.8 ± 1.8  & 53.8 ± 1.8          \\ \cline{2-7} 
%%                                                                               & Pipeline     & 48.5 ± 1.3          & 53.5 ± 1.3 \%          & \textbf{53.7 ± 2.0}    & 53.2 ± 1.4  & 53.2 ± 1.7          \\ \hline
%%\multirow{2}{*}{\begin{tabular}[c]{@{}c@{}}2 minute\\ duration\end{tabular}}   & ROI          & 65.2 ± 1.9          & \textbf{66.2 ± 1.6 \%} & 52.0 ± 2.0 \%          & 58.2 ± 1.9  & 58.0 ± 2.1          \\ \cline{2-7} 
%%                                                                               & Pipeline     & 50.2 ± 0.8          & 52.8 ± 1.5 \%          & \textbf{55.5 ± 1.7}    & 52.3 ± 0.6  & 52.7 ± 1.9          \\ \hline
%%\end{tabular*}%
%%
%%\caption{Results for New Age Group 2}
%%\label{NewAgeGroup2}
%%\end{table*}
%%
%%\subsection{VST Results}
%%%%%%%%%%%%%%%%%%%%%%%%%
%\begin{table*}[]
%	\centering
%	\caption{Gender prediction accuracy over 300 runs using 48 participants in VST (using session 1 data and Velocity threshold = 150)}
%	\label{12sec_start_traj}
%	\begin{tabular*}{0.78\textwidth}{@{\extracolsep{\fill}}|l|llllll|}
%		\hline
%		\multicolumn{7}{|c|}{Different duration from the start of the trajectory lengths \textbf{(Features number is 4)}  }                                                                                                                                                           \\ \hline
%		Time duration                                                                  & Session No. & LogReg              & SVM                    & RF                     & Naive Bayes & RBFN                \\ \hline
%		\multirow{2}{*}{\begin{tabular}[c]{@{}c@{}}12 second\\ \end{tabular}}  & 1          & \textbf{62.4 ± 0.8 } & 53.5 ± 0.7 \%          & 55.6 ± 0.8\%          & 60.9 ± 0.8 \%   & 57.4 ± 0.8  \%          \\ \cline{2-7} 
%		& 4     & 53.9 ± 0.9  \%          & 50.4 ± 0.9 \%            & \textbf{56.5 ± 0.9\%} & 55.2 ± 0.9 \%   & 51.5 ± 0.8 \%           \\ \hline
%		& AVG     &       &       &      &      &          \\ \hline
%		\multirow{2}{*}{\begin{tabular}[c]{@{}c@{}}20 second \\ \end{tabular}} & 1          & 55.2 ± 0.9          & 48.0 ± 0.5 \% & 51.7 ± 0.8 \%          & \textbf{59.0 ± 0.8 \% }  & 50.8 ± 0.7  \%     \\ \cline{2-7} 
%		& 4     & 62.3 ± 0.8 \%          & 55.9 ± 0.7 \%             & 61.2 ± 0.8 \% & \textbf{64.2 ± 0.8} & 59.0 ± 0.8 \%         \\ \hline
%		& AVG     &       &       &      &      &          \\ \hline
%		\multirow{2}{*}{\begin{tabular}[c]{@{}c@{}}40 second\\ \end{tabular}}  & 1          & 47.9 ± 0.9 \%         & 51.9 ± 0.5\%          & \textbf{58.2 ± 0.8\%}         & 54.3 ± 0.7\%  & 54.3 ± 0.7 \% \\ \cline{2-7} 
%		& 4     & 54.0 ± 0.8\%        & 51.4 ± 0.5 \%          & \textbf{56.0 ± 0.8 \%}    & 51.3 ± 0.6\% & 52.5 ± 0.6\%  \%        \\ \hline
%		& AVG     &       &       &      &      &          \\ \hline
%		\multirow{2}{*}{\begin{tabular}[c]{@{}c@{}}1 minute\\ \end{tabular}}   & 1      & \textbf{60.6 ± 0.9 \%} & 53.3 ± 0.7 \% & 56.8 ± 0.7 \%  & 54.7 ± 0.6 \% & 55.0 ± 0.8\%  \\ \cline{2-7} 
%		& 4     & 55.0 ± 0.8 \%        & 51.9 ± 0.5 \%          & \textbf{56.1 ±0.8 }  & 50.3 ± 0.6  & 54.2 ± 0.5\%        \\ \hline
%		& AVG     &       &       &      &      &          \\ \hline
%		\multirow{2}{*}{\begin{tabular}[c]{@{}c@{}}2 minute\\ \end{tabular}}   & 1          & 60.3 ± 0.9 \%  & 55.5 ± 0.7\% & 58.3 ± 0.7\%          & 51.2 ± 0.4\% & \textbf{61.0 ± 0.8\%} \\ \cline{2-7} 
%		& 4     & 56.7 ± 0.9\% & 56.9 ± 0.7\%          & 60.1 ± 0.8\% & 57.9 ± 0.7   & \textbf{62.6 ± 0.7\%}  \\ \hline
%		& AVG     &       &       &      &      &          \\ \hline
%	\end{tabular*}%
%\end{table*}
